# Supplementary material for: Tisane: Authoring Statistical Models via Formal Reasoning from Conceptual and Data Relationships
Source: arXiv:2201.02705 source file (2022-01-07)
Supplement: Supplementary file 2 [file additional_tables_and_figures.tex]

\section{Family and Link functions Tisane currently supports}
We implemented Tisane using \statsmodels for GLMs without mixed effects and
\pymer for GLMs with mixed effects.~\autoref{tab:tableFamilyLinkFunctions} lists the family and link
functions these libraries currently supports. Tisane can be extended to take
advantage of new family and link implementations in these libraries.

\tableFamilyLinkFunctions



\section{Additional examples of graphs that may be constructed}
\figureComplexModeratesGraphIR
\figureOnlyAssociatesOrCausesEdgesCandidateMainEffects


\section{Cautioning analysts about adding certain kinds of variables}
\figurePossibleConfoundingAssociation
