# Supplementary material for: Tisane: Authoring Statistical Models via Formal Reasoning from Conceptual and Data Relationships
Source: arXiv:2201.02705 source file (2022-01-07)
Supplement: Supplementary file 3 [file causal_analysis_differentiation.tex]

\begin{comment}
\section{How does Tisane compare to formal causal analysis?}
Tisane does not perform formal causal analyses~\cite{pearl1995doCalculus,richardson2013SWIGs,greenland1999causal}.
Linear models are versatile because they can model causal and non-causal
relationships simultaneously. This flexibility, however, presents a challenge in
ensuring the conceptual justifiability of models used for explaining, not just
predicting, data.

To derive conceptually valid statistical models, Tisane borrows the fact that
DAGs used in formal causal analyses encode conditional (in)dependencies. These
conditional (in)dependencies have implications on how linear models that explain
the causal influences on a variable in the graph should be formulated. In a
formal causal DAG, a set of nodes may block, or d-separate, a node (i.e., a
dependent variable) from the rest of the causal graph. This means that the
d-separated nodes are conditionally indepenent from the dependent variable. In
other words, if all the nodes in the graph were included in a linear model as
independent variables to explain the dependent variable, the parameter estimates
of the blocked nodes would be close to 0 while the parameter estimates of the
blocking nodes would not be. However, additional methods are necessary to
account for non-causal relationships that a linear model can explain.
Specifically, associative relationships suggest the presence of hidden
variables, which may mediate the causal effect of a variable on the depdendent
variable or causally influence independent and dependent variables
simultaneously.

One view of the candidate main effect generation process is that the variables
analysts specify in their queries act as an initial set of blocking variables
(or conditioning set). Then, the purpose of candidate main effect generation is
for Tisane to (i) find variables that are d-connected (causal edges) or could be
d-connected (associative edges) to the dependent variable and therefore exert
causal influence on the dependent variable and \as{We don't do this anymore, right, @Eunice?: }(ii) find d-separated causal
ancestors that, if included instead of their children, would minimize
multicollinearity concerns while still accounting for causal influence in the
graph.
\end{comment}


% if graph has only associates edges
% because associations may imply the presence of hidden
% variables that may act on the DV and IVs, perhaps even simultaneously.

\section{How does Tisane relate to Entity-Relationship models?}
Tisane's graph IR is an entity-relationship (ER) model~\cite{chen1976ERDiagram}.
ER models, or diagrams, are used to describe data schema. ER models describe how
entities relate to other entities and attributes. In Tisane, a variable of Unit
type can be viewed as an entity. The \texttt{nests\_within} edge describes how
two units, or entities, relate to one another. Tisane's graph IR also relates
units (entities) to measures (attributes).


% represents units and measures in a way similar to
% entity-relationship (E-R) diagrams, which are used to describe database schema.
% Whereas

% Units are analogous to entities, and measures are analogous to attributes
% describing entities. The primary difference between Tisane's graph represents

% Tisane's graph IR is a type of entity-relationship model~\cite{},
% which are used to describe database schemas. Differing from Chen's originally proposed ER diagram, Tisane's graph representation relates units to measures



% Tisane's relationship entity to relationship diagrams
