# Supplementary material for: Tisane: Authoring Statistical Models via Formal Reasoning from Conceptual and Data Relationships
Source: arXiv:2201.02705 source file (2022-01-07)
Supplement: Supplementary file 4 [file design_process.tex]

\section{Tisane \SDSLlong design process}
Insights from an iterative process informed Tisane's design. We summarize
insights from prior work, informal usability feedback, and a pilot study with an
earlier version of Tisane below. 

\subsection{Formative work}

With Tisane's graph specification language, we aimed to collect the necessary
information to infer a GLM and to provide a straightforward way of collecting
it. We consulted statistical best practices on how to construct valid
GLMs~\cite{kreft1998introducing,barr2013randomUpdated,barr2013random,mcelreath2020statistical},
which led us to two sets of variable relationships: \textit{conceptual
relationships}, specifically about causal and correlational relationships to
explain using a GLM and \textit{data measurement relationships} about the
frequency of observations per observational unit (or ``level'') and how
observations may be clustered (e.g., nesting).

We conducted an exploratory survey of 12 study design and data collection
packages. We identified these libraries using word of mouth and bibliographic
references. Eight libraries %in our sample
focused on the controlling the presentation of stimuli and trials (lower-level).
Five were focused on the distribution of conditions (e.g., within-subjects vs.
between-subjects) and frequency of measures (higher-level). We prototyped
Tisane's \SDSL based on the constructs common across these tools. After
cycles of informal usability critiques of language design and a pilot study, we
settled on Tisane's current API.

\tableStudyDesignTools



\subsection{Pilot study}
To better understand how using variable relationships to author statistical
models affects data analysis workflows, we tested an earlier protoype of Tisane
with three computer science researchers (in AI, HCI, and systems, whom we refer
to as P1, P2, and P3, respectively). We were concerned that we were
redistributing the difficulty of authoring GLMs from specifying them directly
to expressing potentially obscure variable relationships.
% who had experience with programming, exploratory data analysis,
% visualization, hypothesis testing, and linear modeling. Each researcher
% participated in an informative interview, a think-aloud session using Tisane to
% analyze a dataset they had previously collected and analyzed, and a brainstorm,
% lasting 2-3 hours. The pilot study informed changes to Tisane reflected in the
% current version of the system.

All three researchers reported that the \SDSLlong %graph specification language
was
straightforward. P2 remarked, ``The API is very simple and elegant. It's very
intuitive. It gets me really thinking about what's the essential or most
important part of the analysis.'' Needing to explicitly state variable relationships in Tisane prompted P1 and P2
to think more critically about their domain and discover new analysis paths (P1, P2, P3). For
example, Tisane helped P1, who previously had erroneously believed multiple
t-tests with Bonferonni corrections were more appropriate than a GLM
for his data, realize how a GLM could have helped him answer questions
he had not had the foresight to ask beforehand. %This observation corroborated
%our hope for Tisane, so we
We were encouraged to see researchers reap additional benefits of having to
specify variable relationships.

Earlier versions of Tisane had a more
extensive API that distinguished between observations and experimental
treatments and provided multiple ways to specify the same types of
relationships. We observed that the researchers gravitated toward a smaller
subset of language constructs around unit and measure declaration, so we introduced explicit types for
units and measures and removed redundant functions.
