# Supplementary material for: Tisane: Authoring Statistical Models via Formal Reasoning from Conceptual and Data Relationships
Source: arXiv:2201.02705 source file (2022-01-07)
Supplement: Supplementary file 5 [file more_examples.tex]

% \diff{\section{More complex nesting examples}}
% % \ej{Add here, including pointers to code base!}
% More complex examples of nesting can be found on Github: https://github.com/emjun/tisane/tree/main/examples. 

\section{Code repository and more examples}
Tisane is an open-source software package. The latest code and ongoing
developments can be found at https://github.com/emjun/tisane. The repository
contains more examples of input Tisane programs (e.g., with more complex nesting
structures) and output scripts. 

Tisane is available for installation via \texttt{pip}, the popular Python package
manager: \texttt{pip install tisane}.
