# Supplementary material for: Tisane: Authoring Statistical Models via Formal Reasoning from Conceptual and Data Relationships
Source: arXiv:2201.02705 source file (2022-01-07)
Supplement: Supplementary file 6 [file usage_scenario_results.tex]

\section{Usage scenario results}
\def\poundslost{\texttt{pounds\_lost}\xspace}
% \def\motivation{\texttt{motivation\_level}\xspace}
\def\motivation{\texttt{motivation}\xspace}
\def\regimen{\texttt{regimen\_condition}\xspace}
\def\group{\texttt{group}\xspace}
\def\age{\texttt{age}\xspace}

\michaelSecondModelOutput

\bridgetModelOutput
